# Supplementary material for: Carbon Regulation and Competition in the European Airline Industry
Source: arXiv:2603.27724 source file (2026-10-22)
Supplement: Supplementary file 1 [file Appendix_Figures.tex]

\section{Figures}

\begin{figure}[h!]
    \centering
    \includegraphics[width=0.98\textwidth]{full service and low cost.png}
    \caption{Market Share for Different Types of Airlines}
    \label{fig:figure1}
\end{figure}

\clearpage

\begin{figure}[h!]
    \centering
    \begin{subfigure}
        \centering
        \includegraphics[width=0.6\textwidth]{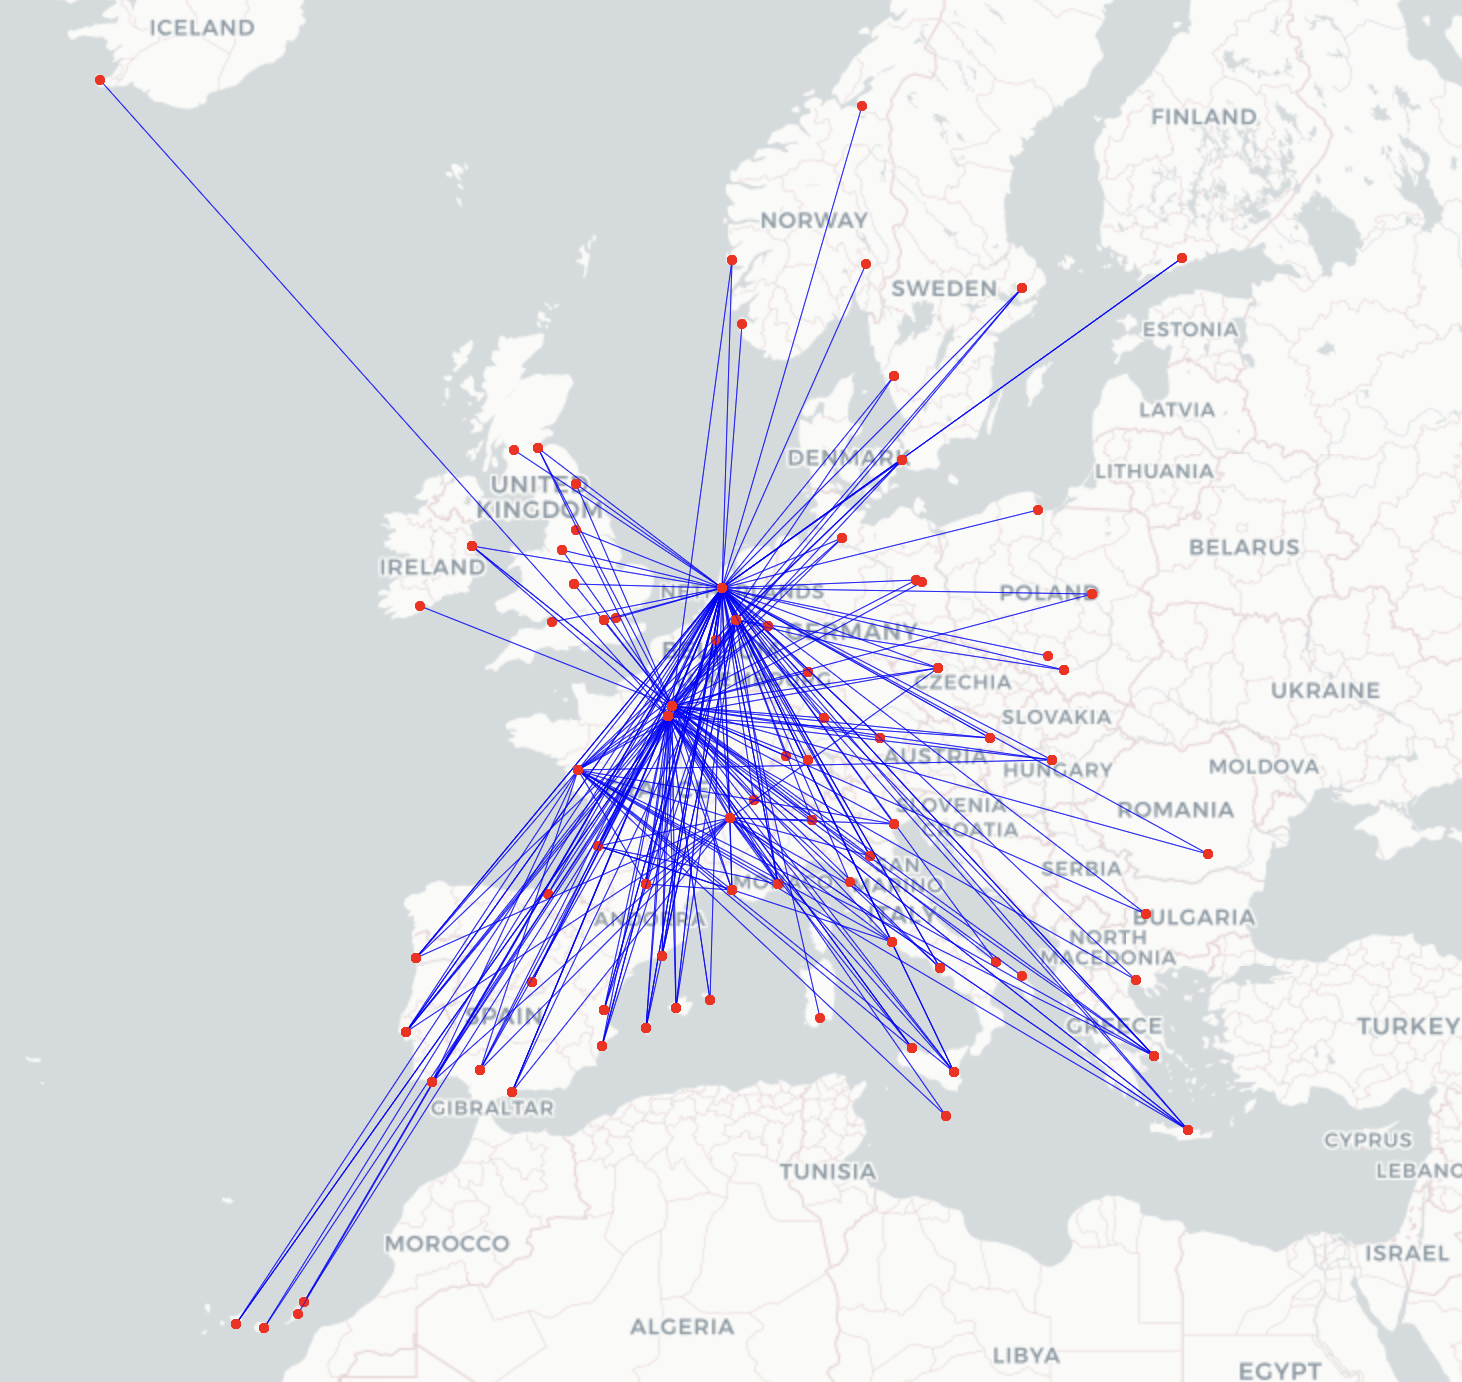}
        \caption{Air France-KLM Group Route Map}
        \label{fig:sub1}
    \end{subfigure}

    \begin{subfigure}
        \centering
        \includegraphics[width=0.6\textwidth]{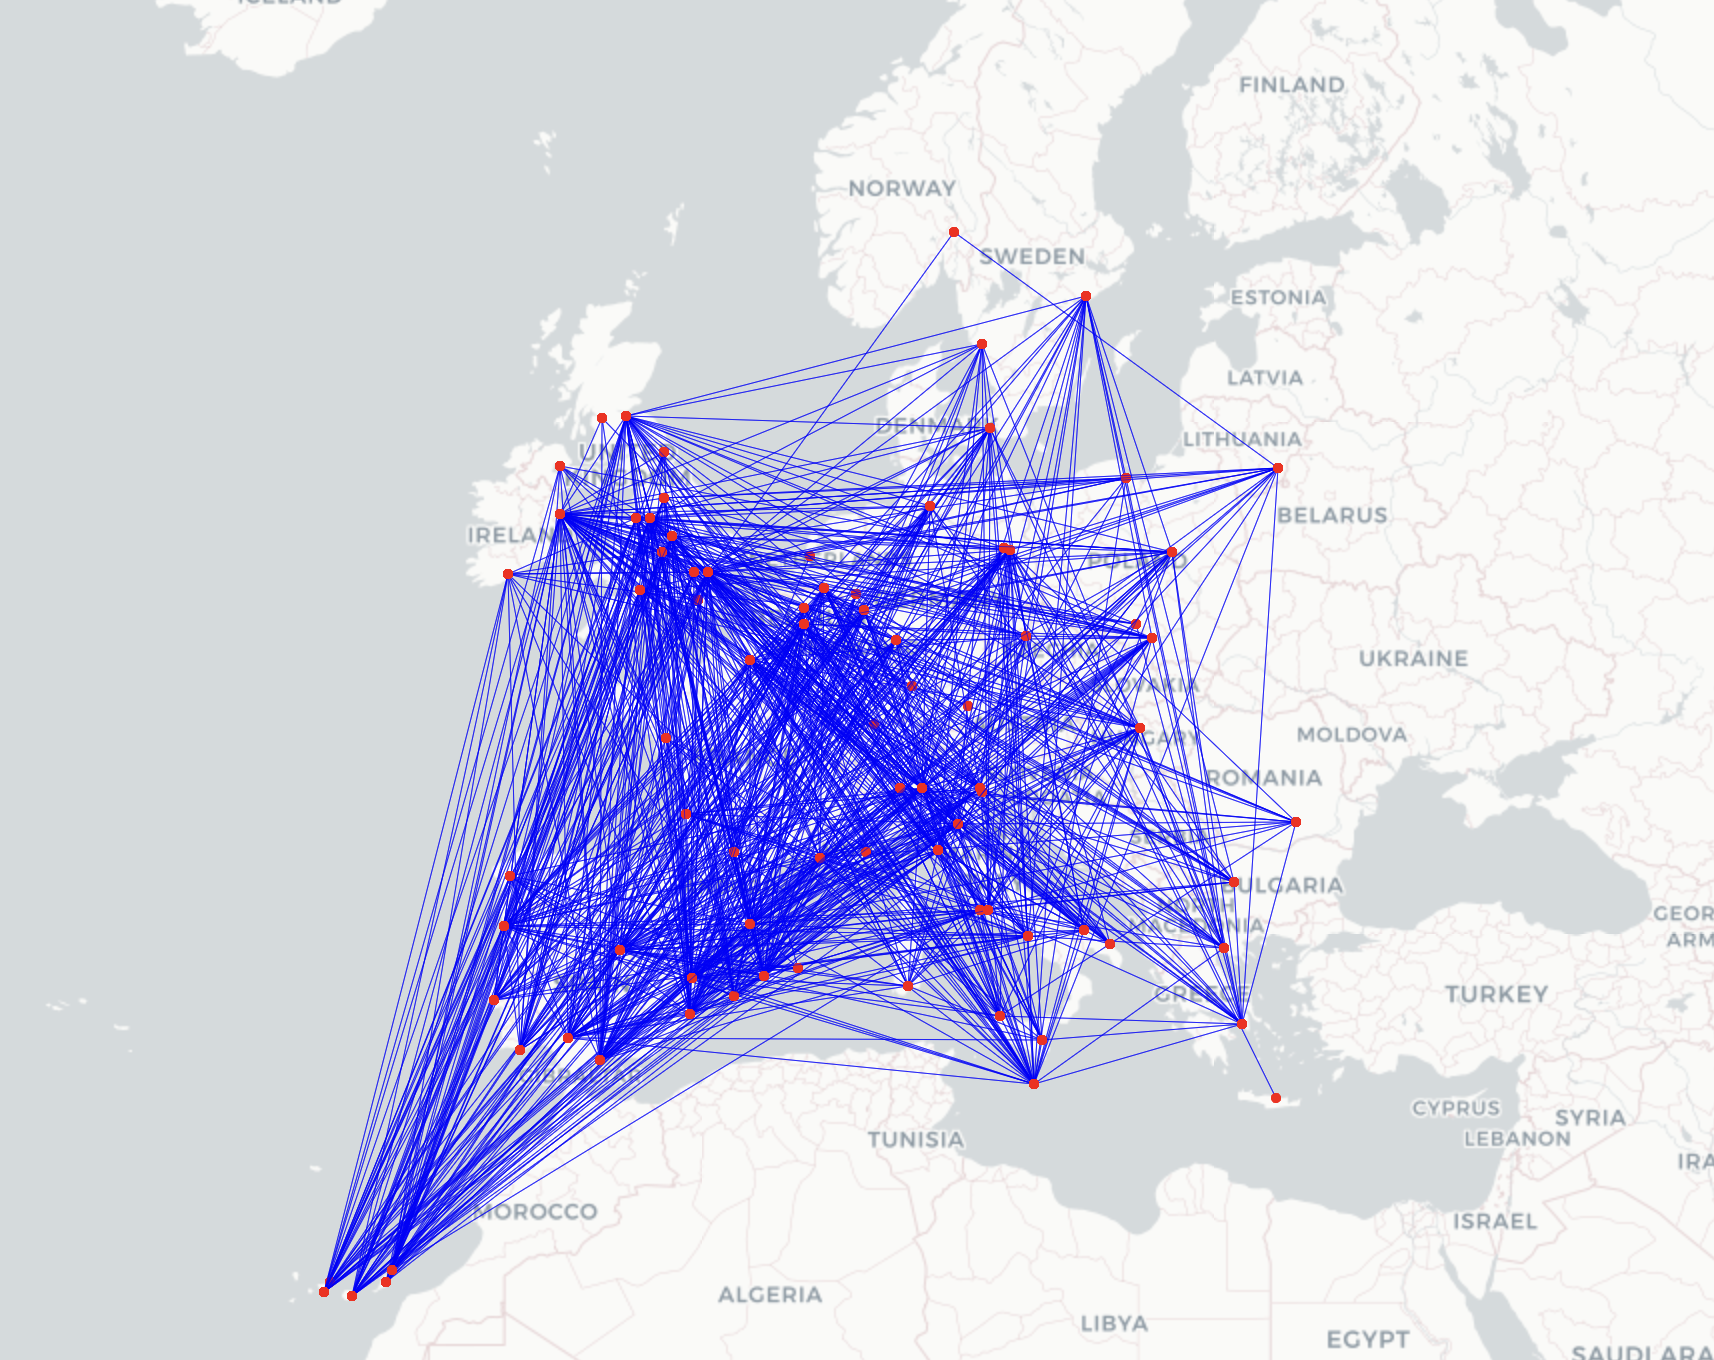}
        \caption{Ryanair Route Map}
        \label{fig:sub2}
    \end{subfigure}

    \caption{Comparing Route Map Between Full-service and Low-cost Airlines}
    \label{fig:figure4}
\end{figure}

\clearpage

\begin{figure}[h!]
    \centering
    \includegraphics[width=0.98\textwidth]{airports diff.png}
    \caption{Proportion of Passengers Travelling from/to at Least one Hub}
    \label{fig:figure5}
\end{figure}

\clearpage

\begin{figure}[h!]
    \centering
    \includegraphics[width=0.98\textwidth]{Num of Parents.png}
    \caption{Number of Airlines in Each Market}
    \label{fig:figure6}
\end{figure}

\clearpage

\begin{figure}[h!]
    \centering
    \includegraphics[width=0.98\textwidth]{num of airline and fare.png}
    \caption{Average Fare vs. Number of Airlines in Each Market}
    \label{fig:figure7}
\end{figure}

\clearpage

\begin{figure}[h!]
    \centering
    \includegraphics[width=0.98\textwidth]{num of routes for hubs.png}
    \caption{Number of Routes Linking at Least One Hub Airport}
    \label{fig:figure8_appendix}
\end{figure}

\clearpage

\begin{figure}[h!]
    \centering
    \begin{subfigure}
        \centering
        \includegraphics[width=0.9\textwidth]{route change for all airlines.png}
        \caption{Quarterly Numbers of Routes Change}
        \label{fig:sub3}
    \end{subfigure}

    \begin{subfigure}
        \centering
        \includegraphics[width=0.9\textwidth]{route change for big airports.png}
        \caption{Quarterly Numbers of Routes Change for Hub Airports}
        \label{fig:sub4}
    \end{subfigure}

    \caption{Comparing Quarterly Numbers of Routes Change}
    \label{fig:figure11}
\end{figure}

\clearpage

\begin{sidewaysfigure}
    \centering
    \includegraphics[width=0.98\textwidth]{figures/different shares.png}
    \caption{Market Share Analysis}
    \label{fig:figure12}
\end{sidewaysfigure}

\clearpage

\begin{sidewaysfigure}
    \centering
    \includegraphics[width=0.98\textwidth]{figures/network density.png}
    \caption{Network Analysis}
    \label{fig:figure13}
\end{sidewaysfigure}

\clearpage

\begin{figure}[h!]
    \centering
    \begin{subfigure}
        \centering
        \includegraphics[width=0.8\textwidth]{Xi plot.png}
        \caption{$\xi$ Plot for BA (IAG Group)}
        \label{fig:sub5}
    \end{subfigure}

    \begin{subfigure}
        \centering
        \includegraphics[width=0.8\textwidth]{Xi plot 2.png}
        \caption{$\xi$ Plot for FR (Ryanair)}
        \label{fig:sub6}
    \end{subfigure}

    \caption{$\xi$ Plot for Two Representative Airlines}
    \label{fig:figure16}
\end{figure}

\clearpage

\begin{figure}[h!]
    \centering
    \begin{subfigure}
        \centering
        \includegraphics[width=0.7\textwidth]{own price elasticity.png}
        \caption{Own-Price Elasticity Plot}
        \label{fig:sub7}
    \end{subfigure}

    \begin{subfigure}
        \centering
        \includegraphics[width=0.7\textwidth]{cross price elasticity.png}
        \caption{Cross-Price Elasticity Plot}
        \label{fig:sub8}
    \end{subfigure}

    \caption{Price Elasticity Plot}
    \label{fig:figure19}
\end{figure}

\clearpage
